# Supplementary material for: Observation of extrinsic topological phases in Floquet photonic lattices
Source: arXiv:2412.14324 ancillary file (2024-12-18)
Supplement: Supplementary file 1 [file Extrinsic_topology_suppl.pdf]

# Supplemental Material: Observation of extrinsic topological phases in Floquet photonic lattices

Rajesh Asapanna,[1,*] Rabih El Sokhen,[1,*] Albert F. Adiyatullin,[1,†]
Clément Hainaut,[1] Pierre Delplace,[2] Álvaro Gómez-León,[3,‡] and Alberto Amo[1,§]

[1] *Univ. Lille, CNRS, UMR 8523 – PhLAM – Physique des Lasers Atomes et Molécules, F-59000 Lille, France*
[2] *ENS de Lyon, CNRS, Laboratoire de Physique (UMR CNRS 5672), F-69342 Lyon, France*
[3] *Institute of Fundamental Physics IFF-CSIC, Calle Serrano 113b, 28006 Madrid, Spain*

(Dated: December 16, 2024)

## CONTENTS

Experimental set-up 2

Computation of the Berry curvature and Chern numbers 2

Discrete-step Floquet operators in Real space 4

Discrete-step Floquet operators and Eigenvectors in reciprocal space 9
Eigenvalues and eigenvectors 10

Computation of the winding of the edge operators 10

Computation of the winding of the stripe operators in the bulk 13

Edge modes in real space 17

References 17

## EXPERIMENTAL SET-UP

The experimental setup employs a continuous wave (CW) single-frequency laser source (Koheras MIKRO, NKT Photonics) operating at 1550 nm with a maximum output power of 40 mW and a linewidth $< 0.1$ kHz. The laser output is split equally using a 50/50 beam splitter, with one part serving as input to a local oscillator and the other being modulated into 1.4 ns pulses via an electro-optical modulator (EOM, iXblue MXER-LN-10), which is controlled by an arbitrary waveform generator (AWG 7000B, Tektronix). To reduce residual laser light entering the ring, an acoustic optical modulator (AOM, AA Opto-electronic MT110-IIR30-Fio-PM0.5) with an extinction power of -70 dB is incorporated. The AOM is shaped in a gate centred in time at the pulse generated by the preceding EOM. The prepared injection signal is then introduced into the long $\alpha$ ring through a 70/30 beamsplitter.

The pulse evolution follows a split step walk. The two fiber rings $\alpha$ and $\beta$ are coupled via a high-bandwidth 40 GHz electronically controlled variable beamsplitter (EOSpace AX-2x2-0MSS-20). Each ring has an Erbium-doped fiber amplifier (EDFA, Keopsys CEFA-C-HG) and an optical variable attenuator (VOA, Agiltron) which are used to finely compensate for round trip losses.

A 90/10 beamsplitter within each ring extracts light for measurement. To access both amplitude and phase information of sublattices $\alpha_n^m$ and $\beta_n^m$, a heterodyne measurement technique is employed. This involves beating the wavefield extracted from the double rings with a local oscillator reference field. This field is derived from the laser used to inject the initial pulse and is frequency-shifted by 3 GHz using an electro-optic modulator. The beating interference between the signal and the local oscillator is converted to electrical signals using a fast photodiode (Thorlabs DET08CFC) operating at 5 GHz. These signals are then captured and analyzed using a high-performance oscilloscope (Tektronix MSO64) featuring a 6 GHz bandwidth, 10-bit vertical resolution, 25 GS/s sampling rate, and a memory record length of 62.5 Mpts corresponding to 2.5 ms, enabling very detailed signal analysis of the beating.

## COMPUTATION OF THE BERRY CURVATURE AND CHERN NUMBERS

To compute the Berry curvature, the eigenvectors of our lattice need to be accessed experimentally. Data is collected by recording the output intensity from both fiber loops using an oscilloscope. The resulting signal displays groups of pulses separated by the average round-trip time of $\bar{T} = 224.94$ ns, with pulses within each group spaced $\Delta T = 3.4$ ns apart due to the length difference between the two fiber loops as shown in Fig. S1.**a**. This time trace is then segmented and arranged into a spatio-temporal diagram (Fig. S1.**b**) for further analysis. Crucial phase information is retrieved by subjecting the signal to optical heterodyne measurement with a reference continuous wave laser, frequency-shifted by about 3 GHz, producing observable fringes in the recorded signal.

The interference between the local oscillator and the signal evolving in the rings contains phase information relevant to the measurement of the band structure (see the beating signal on top of each pulse in Fig. S1.**b**). The band structure is reconstructed by performing a numerical two-dimensional Fourier transform (2DFT) on the stroboscopic spatio-temporal diagram of Fig. S1.**b** of each ring at time steps corresponding to integer Floquet periods ($m = 4, 8, 12, \cdots$). This yields periodic eigenvalue bands spanning 25 GHz in the quasimomentum direction and 1.12 MHz in the quasienergy direction. We focus on a single Brillouin zone at around a frequency of 3GHz as shown in Fig. S1.**c**.

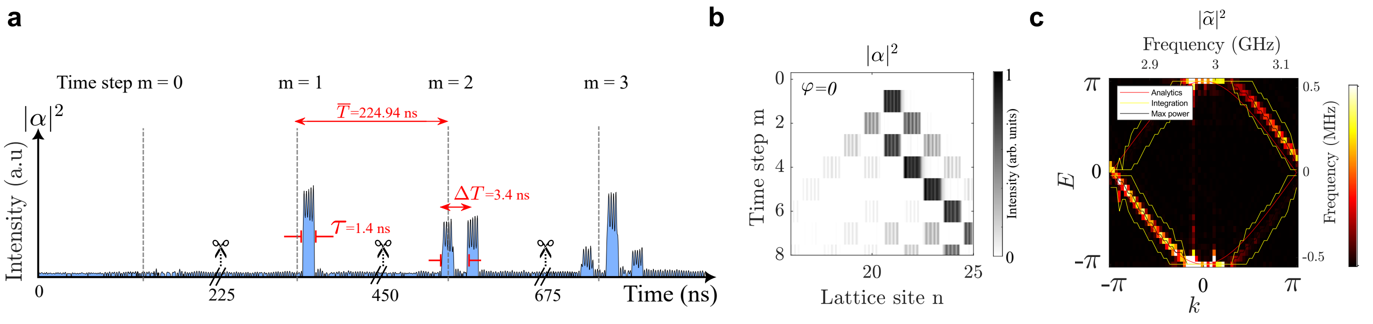


FIG. S1. **a** Zoom on the first time steps of the measured time trace of the signal intensity at the output of the $\alpha$ fiber loop. **b** Spatio-temporal diagram of the $\alpha$ ring reconstructed from the time trace in **a**. **c** Two-dimensional Fourier transform (2DFT) on the stroboscopic spatio-temporal diagram of $\alpha$ ring and Measured bands in one Brillouin zone.

However, environmental factors can cause fluctuations in fiber length, resulting in shifts of the band structure. To diminish these fluctuations we use a protocol using piezos to lock the lengths of the rings. Even after this compensation we still have slight shifts in band structure. To compensate for these minor shifts, the experimental setup employs a dual-pulse technique to reconstruct and calibrate the two-dimensional band structure of our synthetic lattice created using coupled fiber rings.

This method utilizes two consecutive $\tau = 1.4$ ns pulses: a calibration pulse and a science pulse. The calibration pulse, enters the ring and evolves in time with a constant splitting of 50/50 in the variable beamsplitter and no phase modulation. The spatio-temporal evolution dynamics produces a well-known reference band structure. In contrast, the science pulse implements the experimental system of interest, featuring controlled coupling values of variable beamsplitter and phase modulation of phase modulator. The calibration pulse's band structure is compared to its theoretical model, allowing for the measurement of horizontal and vertical shifts. These measurements are then used to calibrate the axes, which remain valid for the subsequent science pulse measurement.

For eigenvector extraction, first, for each quasimomentum value, the experimental bands are identified by scanning around the analytically computed bands to locate intensity maxima. Next, the complex amplitudes $\tilde{\alpha}$ and $\tilde{\beta}$ of the measured bands are obtained at each quasimomentum point for both the $\alpha$ and $\beta$ rings. From them we extract the amplitude ratio $R(k, \varphi)$ between $\tilde{\alpha}$ and $\tilde{\beta}$ and their phase difference $\Phi_{\alpha\beta}(k, \varphi)$. To reduce noise in the measurement of the amplitude ratio $R$, the recorded intensity is integrated over a small range surrounding the band maximum for each $k$ value as shown in Fig. S1.**c**. This ratio $R$ and the phase difference $\Phi_{\alpha\beta}$ of the complex amplitudes directly yield the eigenvectors.

Again the calibration shot is crucial for establishing a consistent phase reference across different measurements; specifically, the phase is rigidly shifted to zero at $k = -\pi$ in the calibration shot, and this shift is applied to the science shot. The sublattice phase pattern $\Phi_{\alpha\beta}(k, \varphi)$ is then reconstructed from independent measurements taken at various values of $\varphi \in [-\pi, \pi]$, utilizing the calibration shot as a reference. To obtain the final eigenvectors $|\psi\rangle$ defined by Equation S1 smoothing is applied to the resulting matrices $|R(k, \varphi)|$ and $\Phi_{\alpha\beta}(k, \varphi)$:

$$|\psi\rangle = \begin{pmatrix} \tilde{\alpha}(k,\varphi) \\ \tilde{\beta}(k,\varphi) \end{pmatrix} = \frac{1}{\sqrt{1 + |R(k,\varphi)|^2}} \begin{pmatrix} 1 \\ |R(k,\varphi)| e^{i\Phi_{\alpha\beta}(k,\varphi)} \end{pmatrix} \tag{S1}$$

where,

$$R(k,\varphi) = \frac{\tilde{\beta}(k,\varphi)}{\tilde{\alpha}(k,\varphi)} = |R(k,\varphi)| e^{i\Phi_{\alpha\beta}(k,\varphi)} \tag{S2}$$

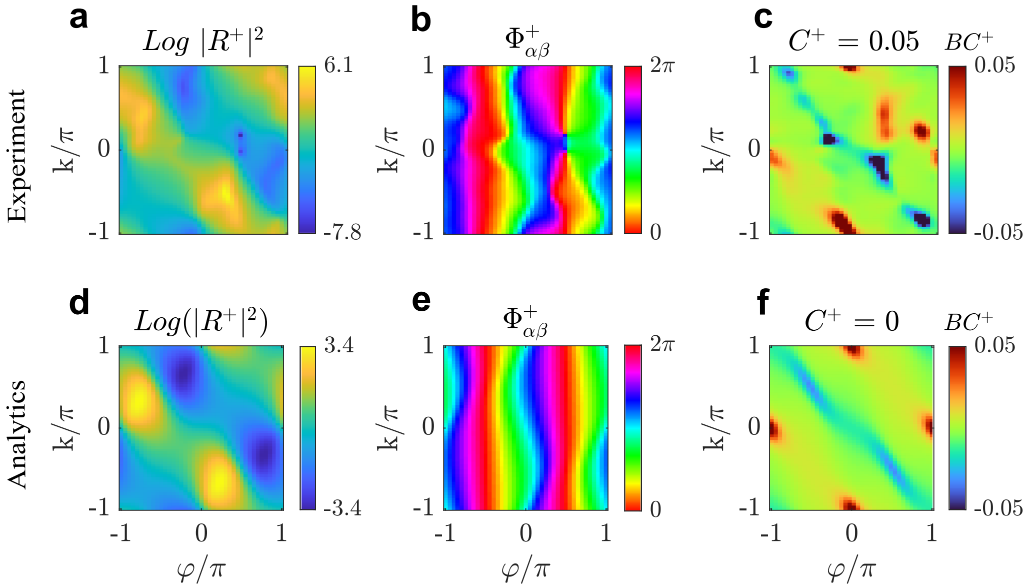


FIG. S2. **Chern Number $\mathcal{C}^+ = 0$** for the upper band of the model with $\theta_1 = 0.125\pi$, $\theta_2 = 0.25\pi$, $\theta_3 = 0.438\pi$ and $\theta_4 = 0.438\pi$. Experimental relative amplitude and phase difference between the two sublattices for the eigenvectors are shown in **a, b** and their corresponding analytical calculations in **d, e**. **c** Measured Berry curvature of the upper band for this lattice model and corresponding measured Chern number shown on top. **f** Theoretical Berry curvature of the upper band for this lattice model and corresponding Chern number shown on top.

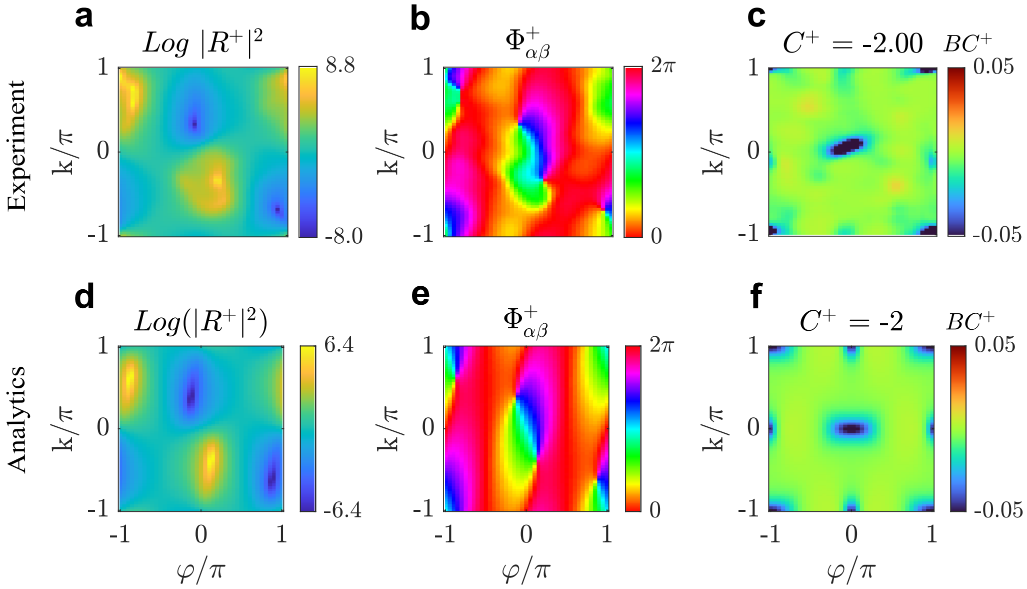


FIG. S3. **Chern Number $\mathcal{C}^+$ = -2** for the upper band of the model with $\theta_1 = 0.125\pi$, $\theta_2 = 0.25\pi$, $\theta_3 = 0.5\pi$ and $\theta_4 = 0.25\pi$. Experimental relative amplitude and phase difference between the two sublattices for the eigenvectors are shown in **a, b** and their corresponding analytical calculations in **d, e**. **c** Measured Berry curvature of the upper band for this lattice model and corresponding measured Chern number shown on top. **f** Theoretical Berry curvature of the upper band for this lattice model and corresponding Chern number shown on top.

Figures S2.**a-b** and S3.**a-b** show the experimentally measured $|R(k,\varphi)|$ and $\Phi_{\alpha\beta}(k,\varphi)$ for the upper band corresponding to the two cases with $\mathcal{C} = 0$ and 2 described in Figs. 3 and 4 of the main text. Panels **d** and **e** show the corresponding analytical calculation using Equation S36. We can now compute the Berry curvature using the measured eigenvectors.

The Berry curvature is computed utilizing the natural discretization of the Brillouin zone derived from the experimental data. The calculation involves the product of eigenvectors of a given band at the four corners of each square in the discretized Brillouin zone. The four-points formula is used to compute the Berry curvature (or Berry phase) per unit cell for each plaquette of the discretization [1]:

$$BC = -\text{Im}\ \log\left[\langle\psi_1|\psi_2\rangle\langle\psi_2|\psi_3\rangle\langle\psi_3|\psi_4\rangle\langle\psi_4|\psi_1\rangle\right] \tag{S3}$$

where $|\psi_i\rangle$ represents the eigenvector at each corner of the square.

The Chern number is determined by integrating the Berry curvature over the entire Brillouin zone:

$$C = \frac{1}{2\pi}\sum_{BZ} BC \tag{S4}$$

The Chern number is a bulk topological invariant which provides crucial information about the global properties of the lattice, band structure and associated wavefunctions. In Figs. S2 and S3 we show the experimentally measured Chern number in panel **c** and their corresponding analytical calculation in panel **f**.

## DISCRETE-STEP FLOQUET OPERATORS IN REAL SPACE

The discrete-step walk generated by the experimental setup is described by the general coupled equations. Equation S5 is a more general form of Equation (1) of the main text.

$$\begin{aligned}\alpha(n,m+1) &= e^{i\varphi(n-1,m)}(\cos(\theta(n-1,m))\alpha(n-1,m) + i\sin(\theta(n-1,m))\beta(n-1,m))\\ \beta(n,m+1) &= \cos(\theta(n+1,m))\beta(n+1,m) + i\sin(\theta(n+1,m))\alpha(n+1,m)\end{aligned} \tag{S5}$$

It shows how the original pulse splits at each time-step $m$ depending on the value of the variable beam splitter $\theta$ and acquires a phase due to the phase modulator $\varphi$ acting on the $\alpha$ ring. $\alpha(n,m)$ and $\beta(n,m)$ are the complex amplitudes

of light pulses in the long and short rings respectively. The system can be understood as a one dimensional quantum walk with a parametric dimension $\varphi$.

To describe the light dynamics after four time steps, we replace $m$ with $m+3$ in Equation S5. We then iterate Equation S5 to relate the complex amplitudes of $\alpha$ and $\beta$ at time step $m$ to those at time step $m+3$. For our four-step protocol, the final equations of motion describing the time evolution during each full period are given by:

$$
\begin{aligned}
\alpha(n,m+4) = {} & (e^{i\varphi(n-1,m+3)}e^{i\varphi(n-2,m+2)}e^{i\varphi(n-3,m+1)}e^{i\varphi(n-4,m)}T(n-4,m)T(n-1,m+3)\\
& \times T(n-2,m+2)T(n-3,m+1))\alpha(n-4,m)\\
& + (ie^{i\varphi(n-1,m+3)}e^{i\varphi(n-2,m+2)}e^{i\varphi(n-3,m+1)}e^{i\varphi(n-4,m)}R(n-4,m)T(n-1,m+3)\\
& \times T(n-2,m+2)T(n-3,m+1))\beta(n-4,m)\\
& + (-e^{i\varphi(n-1,m+3)}e^{i\varphi(n-2,m+2)}e^{i\varphi(n-3,m+1)}R(n-2,m)R(n-3,m+1)T(n-1,m+3)T(n-2,m+2)\\
& - e^{i\varphi(n-1,m+1)}e^{i\varphi(n-1,m+3)}e^{i\varphi(n-2,m)}R(n,m+2)T(n-2,m)R(n-1,m+3)T(n-1,m+1)\\
& - e^{i\varphi(n-1,m+3)}e^{i\varphi(n-2,m+2)}e^{i\varphi(n-2,m)}T(n-2,m)R(n-1,m+1)R(n-2,m+2)T(n-1,m+3))\alpha(n-2,m)\\
& + (ie^{i\varphi(n-1,m+3)}e^{i\varphi(n-2,m+2)}e^{i\varphi(n-3,m+1)}T(n-2,m)R(n-3,m+1)T(n-1,m+3)T(n-2,m+2)\\
& - ie^{i\varphi(n-1,m+3)}e^{i\varphi(n-2,m+2)}e^{i\varphi(n-2,m)}R(n-2,m)R(n-1,m+1)R(n-2,m+2)T(n-1,m+3)\\
& - ie^{i\varphi(n-1,m+1)}e^{i\varphi(n-1,m+3)}e^{i\varphi(n-2,m)}R(n,m+2)R(n-2,m)R(n-1,m+3)T(n-1,m+1))\beta(n-2,m)\\
& + (e^{i\varphi(n-1,m+1)}e^{i\varphi(n-1,m+3)}R(n,m)R(n,m+2)R(n-1,m+1)R(n-1,m+3)\\
& - e^{i\varphi(n-1,m+3)}e^{i\varphi(n,m)}T(n,m)T(n,m+2)R(n+1,m+1)R(n-1,m+3)\\
& - e^{i\varphi(n-1,m+3)}e^{i\varphi(n-2,m+2)}R(n,m)R(n-2,m+2)T(n-1,m+1)T(n-1,m+3))\alpha(n,m)\\
& + (ie^{i\varphi(n-1,m+3)}e^{i\varphi(n-2,m+2)}T(n,m)R(n-2,m+2)T(n-1,m+1)T(n-1,m+3)\\
& - ie^{i\varphi(n-1,m+3)}e^{i\varphi(n,m)}R(n,m)T(n,m+2)R(n+1,m+1)R(n-1,m+3)\\
& - ie^{i\varphi(n-1,m+1)}e^{i\varphi(n-1,m+3)}T(n,m)R(n,m+2)R(n-1,m+1)R(n-1,m+3))\beta(n,m)\\
& + (-e^{i\varphi(n-1,m+3)}R(n+2,m)T(n,m+2)R(n-1,m+3)T(n+1,m+1))\alpha(n+2,m)\\
& + (ie^{i\varphi(n-1,m+3)}T(n,m+2)T(n+2,m)R(n-1,m+3)T(n+1,m+1))\beta(n+2,m)\\
\\
\beta(n,m+4) = {} & (ie^{i\varphi(n-1,m+1)}e^{i\varphi(n,m+2)}e^{i\varphi(n-2,m)}T(n,m+2)T(n-2,m)R(n+1,m+3)T(n-1,m+1))\alpha(n-2,m)\\
& + (-e^{i\varphi(n-1,m+1)}e^{i\varphi(n,m+2)}e^{i\varphi(n-2,m)}R(n-2,m)T(n,m+2)R(n+1,m+3)T(n-1,m+1))\beta(n-2,m)\\
& + (ie^{i\varphi(n+1,m+1)}e^{i\varphi(n,m)}T(n,m)R(n+2,m+2)T(n+1,m+1)T(n+1,m+3)\\
& - ie^{i\varphi(n-1,m+1)}e^{i\varphi(n,m+2)}R(n,m)T(n,m+2)R(n-1,m+1)R(n+1,m+3)\\
& - ie^{i\varphi(n,m)}e^{i\varphi(n,m+2)}T(n,m)R(n,m+2)R(n+1,m+1)R(n+1,m+3))\alpha(n,m)\\
& + (e^{i\varphi(n,m)}e^{i\varphi(n,m+2)}R(n,m)R(n,m+2)R(n+1,m+1)R(n+1,m+3)\\
& - e^{i\varphi(n+1,m+1)}e^{i\varphi(n,m)}R(n,m)R(n+2,m+2)T(n+1,m+1)T(n+1,m+3)\\
& - e^{i\varphi(n-1,m+1)}e^{i\varphi(n,m+2)}T(n,m)T(n,m+2)R(n-1,m+1)R(n+1,m+3))\beta(n,m)\\
& + (ie^{i\varphi(n+2,m)}T(n+2,m)R(n+3,m+1)T(n+1,m+3)T(n+2,m+2)\\
& - ie^{i\varphi(n,m+2)}R(n,m+2)R(n+2,m)R(n+1,m+3)T(n+1,m+1)\\
& - ie^{i\varphi(n+1,m+1)}R(n+2,m)R(n+1,m+1)R(n+2,m+2)T(n+1,m+3))\alpha(n+2,m)\\
& + (-e^{i\varphi(n,m+2)}R(n,m+2)T(n+2,m)R(n+1,m+3)T(n+1,m+1)\\
& - e^{i\varphi(n+2,m)}R(n+2,m)R(n+3,m+1)T(n+1,m+3)T(n+2,m+2)\\
& - e^{i\varphi(n+1,m+1)}T(n+2,m)R(n+1,m+1)R(n+2,m+2)T(n+1,m+3))\beta(n+2,m)\\
& + (iR(n+4,m)T(n+1,m+3)T(n+2,m+2)T(n+3,m+1))\alpha(n+4,m)\\
& + (T(n+4,m)T(n+1,m+3)T(n+2,m+2)T(n+3,m+1))\beta(n+4,m)
\end{aligned}
\tag{S6}
$$

where $T(n,m) = \cos(\theta(n,m))$ and $R(n,m) = \sin(\theta(n,m))$.

In the four-step model, the coupling angle $\theta$ and phase modulator $\varphi$ have a cyclic behaviour, each alternating between four distinct values within a single Floquet period $T_F$. The four-step model exhibits double periodicity: spatial (every two sites $n$ i.e. sites 0, 2, 4, 6, $\cdots$) and temporal (every four-time steps $m$ i.e. steps 4, 8, 12, $\cdots$) as shown in Fig. S5. Therefore, in Eqs. S6 we fix the angles at different times $m$ and sites $n$ to

$$\begin{aligned}&\theta(n,m)=\theta_{1,n}=\theta_1,\ \theta(n,m+1)=\theta_{2,n}=\theta_2,\ \theta(n,m+2)=\theta_{3,n}=\theta_3,\ \theta(n,m+3)=\theta_{4,n}=\theta_4\\&\varphi(n,m)=\varphi_{1,n}=+\varphi,\ \varphi(n,m+1)=\varphi_{2,n}=-\varphi,\ \varphi(n,m+2)=\varphi_{3,n}=+\varphi,\ \varphi(n,m+3)=\varphi_{4,n}=-\varphi\end{aligned}\tag{S7}$$

This means that for a time step $m$ all the coupling ratios and phase modulation are constant throughout the lattice, inn a sequence that is repeated every four steps. In these conditions, Eq. S6 simplifies to,

$$\begin{aligned}\alpha(n,m+4)=&\,T_1T_2T_3T_4\,\alpha(n-4,m)+R_1T_2T_3T_4i\,\beta(n-4,m)\\&-(R_2R_3T_1T_4e^{i\varphi}+R_1R_2T_3T_4e^{-i\varphi}+R_3R_4T_1T_2e^{-i\varphi})\,\alpha(n-2,m)\\&-(R_1R_2R_3T_4ie^{i\varphi}+R_1R_3R_4T_2ie^{-i\varphi}-R_2T_1T_3T_4ie^{-i\varphi})\,\beta(n-2,m)\\&-(R_1R_3T_2T_4+R_2R_4T_1T_3-R_1R_2R_3R_4e^{-2i\varphi})\,\alpha(n,m)\\&-(R_1R_2R_4T_3i-R_3T_1T_2T_4i+R_2R_3R_4T_1ie^{-2i\varphi})\,\beta(n,m)\\&-R_1R_4T_2T_3e^{-i\varphi}\alpha(n+2,m)+R_4T_1T_2T_3ie^{-i\varphi}\,\beta(n+2,m)\\ \beta(n,m+4)=&\,T_1T_2T_3T_4\,\beta(n+4,m)+R_1T_2T_3T_4i\,\alpha(n+4,m)\\&-(R_1R_2T_3T_4e^{i\varphi}+R_3R_4T_1T_2e^{i\varphi}+R_2R_3T_1T_4e^{-i\varphi})\,\beta(n+2,m)\\&-(R_1R_3R_4T_2ie^{i\varphi}+R_1R_2R_3T_4ie^{-i\varphi}-R_2T_1T_3T_4ie^{i\varphi})\,\alpha(n+2,m)\\&-(R_1R_3T_2T_4+R_2R_4T_1T_3-R_1R_2R_3R_4e^{2i\varphi})\,\beta(n,m)\\&-(R_1R_2R_4T_3i-R_3T_1T_2T_4i+R_2R_3R_4T_1ie^{2i\varphi})\,\alpha(n,m)\\&-R_1R_4T_2T_3e^{i\varphi}\beta(n-2,m)+R_4T_1T_2T_3ie^{i\varphi}\,\alpha(n-2,m)\end{aligned}\tag{S8}$$

where $T_j=\cos(\theta_j)$ and $R_j=\sin(\theta_j)$ with $j=1$, 2, 3 and 4.

For an infinite lattice (i.e., a system without boundaries) under the four-step protocol, the full Floquet operator $U_{F,\infty}$ is defined by Eq. S8. This operator characterizes the evolution of the infinite lattice in real space, incorporating spatially couplings $\theta$, phase modulations $\varphi$, and its periodic temporal modulation. The operator $U_{F,\infty}$ can be expressed as:

$$U_{F,\infty}=\begin{pmatrix}\ddots & U_+ & U_{++} & 0 & 0 & 0 & 0 & \iddots\\ U_- & U_0 & U_+ & U_{++} & 0 & 0 & 0 & 0\\ U_{--} & U_- & U_0 & U_+ & U_{++} & 0 & 0 & 0\\ 0 & U_{--} & U_- & U_0 & U_+ & U_{++} & 0 & 0\\ 0 & 0 & U_{--} & U_- & U_0 & U_+ & U_{++} & 0\\ 0 & 0 & 0 & U_{--} & U_- & U_0 & U_+ & U_{++}\\ 0 & 0 & 0 & 0 & U_{--} & U_- & U_0 & U_+\\ \iddots & 0 & 0 & 0 & 0 & U_{--} & U_- & \ddots\end{pmatrix}\tag{S9}$$

the different blocks are given by:

$$U_0=\begin{pmatrix}R_1R_2R_3R_4\mathrm{e}^{-2i\varphi}-R_2R_4T_1T_3-R_1R_3T_2T_4 & R_3T_1T_2T_4i-R_1R_2R_4T_3i-R_2R_3R_4T_1i\mathrm{e}^{-2i\varphi}\\ R_3T_1T_2T_4i-R_1R_2R_4T_3i-R_2R_3R_4T_1i\mathrm{e}^{2i\varphi} & R_1R_2R_3R_4\mathrm{e}^{2i\varphi}-R_2R_4T_1T_3-R_1R_3T_2T_4\end{pmatrix}\tag{S10}$$

$$U_+=\begin{pmatrix}-R_1R_4T_2T_3e^{-i\varphi} & R_4T_1T_2T_3ie^{-i\varphi}\\ R_2T_1T_3T_4ie^{i\varphi}-R_1R_2R_3T_4ie^{-i\varphi}-R_1R_3R_4T_2ie^{i\varphi} & -R_1R_2T_3T_4e^{i\varphi}-R_3R_4T_1T_2e^{i\varphi}-R_2R_3T_1T_4e^{-i\varphi}\end{pmatrix}\tag{S11}$$

$$U_{++}=\begin{pmatrix}0 & 0\\ R_1T_2T_3T_4i & T_1T_2T_3T_4\end{pmatrix}\tag{S12}$$

$$U_- = \begin{pmatrix} -R_2R_3T_1T_4\mathrm{e}^{i\varphi} - R_1R_2T_3T_4\mathrm{e}^{-i\varphi} - R_3R_4T_1T_2\mathrm{e}^{-i\varphi} & R_2T_1T_3T_4i\mathrm{e}^{-i\varphi} - R_1R_3R_4T_2i\mathrm{e}^{-i\varphi} - R_1R_2R_3T_4i\mathrm{e}^{i\varphi} \\ R_4T_1T_2T_3i\mathrm{e}^{i\varphi} & -R_1R_4T_2T_3\mathrm{e}^{i\varphi} \end{pmatrix} \tag{S13}$$

$$U_{--} = \begin{pmatrix} T_1T_2T_3T_4 & R_1T_2T_3T_4i \\ 0 & 0 \end{pmatrix} \tag{S14}$$

The eigenvectors of the infinite lattice $|\Psi\rangle$ are expressed in the basis of $\{\alpha, \beta\}$. This lattice configuration exhibits periodic boundary conditions (PBC) in both the spatial dimension $n$ and the synthetic dimension $\varphi$. In this context, the matrix can be interpreted as a unitary representation of a dimerized lattice. The couplings between adjacent dimers are characterized by $U_\pm$, while the couplings between next-nearest neighbouring dimers are represented by $U_{\pm\pm}$.

The four-step model exhibits a temporal periodicity of four steps (i.e. 4, 8, 12, $\cdots$). Consequently, the Floquet evolution operator $U_{F,\infty}$ in real space characterizes the system's state at every fourth time step, denoted as $\bar{m} = m \pmod 4$. The evolution equation can be expressed as:

$$|\Psi\rangle_{\bar{m}+1} = U_{F,\infty} |\Psi\rangle_{\bar{m}} \tag{S15}$$

where

$$|\Psi\rangle_{\bar{m}} = \begin{pmatrix} \vdots \\ \chi_{\bar{m}}(n-2) \\ \chi_{\bar{m}}(n) \\ \chi_{\bar{m}}(n+2) \\ \vdots \end{pmatrix}, \tag{S16}$$

where we define vector $\chi_{\bar{m}}(n)$ for the dimer $(\alpha, \beta)$ such that,

$$\chi_{\bar{m}}(n) = \begin{pmatrix} \alpha(\bar{m}, n) \\ \beta(\bar{m}, n) \end{pmatrix}. \tag{S17}$$

$|\Psi\rangle_{\bar{m}}$ is the vector representing the state of the system in real space at time step $\bar{m}$.

The bulk topology of our lattice, here we refer to it as intrinsic topology, in different regions of the phase diagram of four-step model is well defined by the Chern number $\mathcal{C}$ because our lattice model corresponds to the D symmetry class with particle hole symmetry (refer Eq. S34) [2] as shown in Fig.2**a** of main paper.

To implement open boundary conditions (OBC) and create a spatially finite lattice in dimension $n$, specific angles must be fixed to $\theta = \pi/2$ at the boundary to ensure full reflectance, as illustrated in Fig. S5**a**. The synthetic dimension $\varphi$ retains its periodic boundary condition (PBC). Given the double periodicity of our lattice in the spatial dimension $n$, we consider only the even site positions resulting in a finite lattice of size $N$, as compared with the full lattice with $n = 2N$ sites depicted in Fig. S5**a**. The full reflection condition necessitates that $\theta_{2,-1} = \pi/2$ and $\theta_{4,-1} = \pi/2$ at the left edge (site position $n = -1$), and $\theta_{2,2N+1} = \pi/2$ and $\theta_{4,2N+1} = \pi/2$ at the right edge (site position $n = 2N + 1$). These conditions define the complete four-steps Floquet operator $U_{F,N}$ for the finite system. The full matrix of size $N \times N$ for the four-step model can be expressed as:

$$U_{F,N} = \begin{pmatrix} U_0^L & U_+^L & U_{++} & 0 & 0 & 0 & 0 & \\ U_-^L & U_0 & U_+ & U_{++} & 0 & 0 & \ddots & 0 \\ U_{--} & U_- & U_0 & U_+ & U_{++} & \ddots & 0 & 0 \\ 0 & U_{--} & U_- & U_0 & \ddots & U_{++} & 0 & 0 \\ 0 & 0 & U_{--} & \ddots & U_0 & U_+ & U_{++} & 0 \\ 0 & 0 & \ddots & U_{--} & U_- & U_0 & U_+ & U_{++} \\ 0 & \ddots & 0 & 0 & U_{--} & U_- & U_0 & U_+^R \\ & 0 & 0 & 0 & 0 & U_{--} & U_-^R & U_0^R \end{pmatrix}, \tag{S18}$$

where the blocks modified due to the condition of full reflection at the edges are given by:

$$U_0^L = \begin{pmatrix} R_1R_3\mathrm{e}^{-2i\varphi} - R_2T_1T_3 & -R_3T_1i\mathrm{e}^{-2i\varphi} - R_1R_2T_3i \\ R_3T_1T_2T_4i - R_1R_4T_3i - R_2R_3R_4T_1i\mathrm{e}^{2i\varphi} & R_1R_2R_3R_4\mathrm{e}^{2i\varphi} - R_1R_3T_2T_4 - R_4T_1T_3 \end{pmatrix} \tag{S19}$$

$$U_+^L = \begin{pmatrix} -R_1T_2T_3\mathrm{e}^{-i\varphi} & T_1T_2T_3i\mathrm{e}^{-i\varphi} \\ R_2T_1T_3T_4i\mathrm{e}^{i\varphi} - R_1R_2R_3T_4i\mathrm{e}^{-i\varphi} - R_1R_3R_4T_2i\mathrm{e}^{i\varphi} & -R_1R_2T_3T_4\mathrm{e}^{i\varphi} - R_3R_4T_1T_2\mathrm{e}^{i\varphi} - R_2R_3T_1T_4\mathrm{e}^{-i\varphi} \end{pmatrix} \tag{S20}$$

$$U_-^L = \begin{pmatrix} -R_1T_3T_4\mathrm{e}^{-i\varphi} - R_2R_3T_1T_4\mathrm{e}^{i\varphi} - R_3R_4T_1T_2\mathrm{e}^{-i\varphi} & T_1T_3T_4i\mathrm{e}^{-i\varphi} - R_1R_2R_3T_4i\mathrm{e}^{i\varphi} - R_1R_3R_4T_2i\mathrm{e}^{-i\varphi} \\ R_4T_1T_2T_3i\mathrm{e}^{i\varphi} & -R_1R_4T_2T_3\mathrm{e}^{i\varphi} \end{pmatrix} \tag{S21}$$

$$U_0^R = \begin{pmatrix} R_1R_2R_3R_4\mathrm{e}^{-2i\varphi} - R_1R_3T_2T_4 - R_4T_1T_3 & R_3T_1T_2T_4i - R_1R_4T_3i - R_2R_3R_4T_1i\mathrm{e}^{-2i\varphi} \\ -R_3T_1i\mathrm{e}^{2i\varphi} - R_1R_2T_3i & R_1R_3\mathrm{e}^{2i\varphi} - R_2T_1T_3 \end{pmatrix} \tag{S22}$$

$$U_+^R = \begin{pmatrix} -R_2R_3T_1T_4\mathrm{e}^{i\varphi} - R_1R_2T_3T_4\mathrm{e}^{-i\varphi} - R_3R_4T_1T_2\mathrm{e}^{-i\varphi} & R_2T_1T_3T_4i\mathrm{e}^{-i\varphi} - R_1R_3R_4T_2i\mathrm{e}^{-i\varphi} - R_1R_2R_3T_4i\mathrm{e}^{i\varphi} \\ T_1T_2T_3i\mathrm{e}^{i\varphi} & -R_1T_2T_3\mathrm{e}^{i\varphi} \end{pmatrix} \tag{S23}$$

$$U_-^R = \begin{pmatrix} -R_1R_4T_2T_3\mathrm{e}^{-i\varphi} & R_4T_1T_2T_3i\mathrm{e}^{-i\varphi} \\ T_1T_3T_4i\mathrm{e}^{i\varphi} - R_1R_3R_4T_2i\mathrm{e}^{i\varphi} - R_1R_2R_3T_4i\mathrm{e}^{-i\varphi} & -R_1T_3T_4\mathrm{e}^{i\varphi} - R_3R_4T_1T_2\mathrm{e}^{i\varphi} - R_2R_3T_1T_4\mathrm{e}^{-i\varphi} \end{pmatrix} \tag{S24}$$

The evolution equation of the system in real space at time step $\bar{m} = m \pmod 4$ for a finite lattice of size $N$ can be written as,

$$|\Psi\rangle_{\bar{m}+1} = U_{F,N}\,|\Psi\rangle_{\bar{m}} \tag{S25}$$

where

$$|\Psi\rangle_{\bar{m}} = \begin{pmatrix} \chi_{\bar{m}}(0) \\ \chi_{\bar{m}}(2) \\ \vdots \\ \chi_{\bar{m}}(2N-2) \\ \chi_{\bar{m}}(2N) \end{pmatrix}. \tag{S26}$$

Fig. S4.**c** shows the eigenvalue spectrum of the lattice with Chern number -2 in the upper band calculated from the eigenvalues of $U_{F,N}$. As mentioned above the lattice has PBC along synthetic dimension $\varphi$ and OBC along the real dimention $n$. The spectrum displays two chiral edge modes per edge in $E = 0$ gap. In our experiment we focus only on the left edge. To excite the left edge mode of our system, we prepare $|\Psi\rangle_0$ such that,

$$|\Psi\rangle_0 = \begin{pmatrix} \chi_0(0) \\ \chi_0(2) \\ \vdots \\ \chi_0(2N-2) \\ \chi_0(2N) \end{pmatrix} \tag{S27}$$

with $\chi_0(0) = \begin{pmatrix} 1 \\ 0 \end{pmatrix}$ and $\chi_0(n) = 0\ \forall n \geq 2$. That is, injection at site position $n = 0$ and time step $\bar{m} = 0$ in the $\alpha$ sublattice ($\alpha(\bar{m} = 0, n = 0) = 1$). We let the the system evolve according to the Equation S25. Then, the eigenvector $|\Psi\rangle_{\bar{m}}$ at time step $\bar{m}$ is give by the expression:

$$|\Psi\rangle_{\bar{m}} = U_{F,N}\,|\Psi\rangle_{\bar{m}-1} = (U_{F,N})^{\bar{m}}\,|\Psi\rangle_0\,. \tag{S28}$$

$|\Psi\rangle_{\bar{m}}$ describes the stroboscopic evolution of the system. Figure S7 shows the spatio-temporal non-stroboscopic evolution of the sublattice $\alpha$ when edge of the lattice is excited for given value of $\varphi$. A 2D Fourier transform of the stroboscopic spatio-temporal dynamics of $\alpha$ ring at time steps corresponding to integer Floquet periods ($m = 4, 8, 12, \cdots$) scanned over $\varphi \in [-\pi, \pi]$ produces the band structure with chiral edge mode as shown in Fig. S4.**a**.

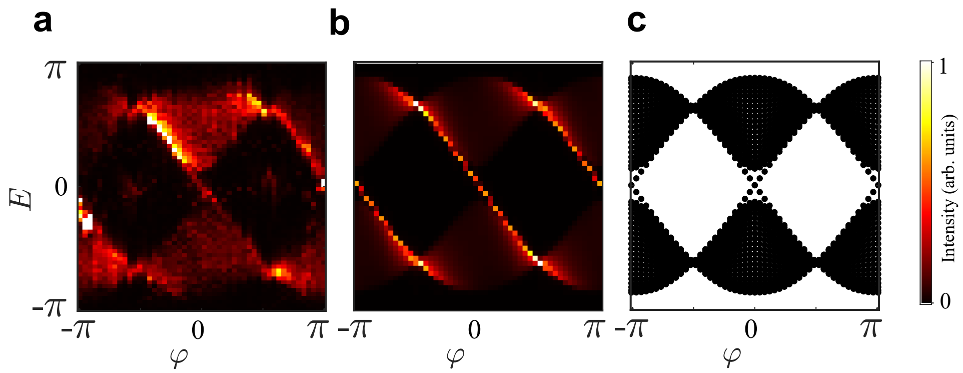


FIG. S4. **Band diagram for a lattice model with Chern number $\mathcal{C}^+$ = -2 and no edge winding i.e. $\nu_{\mathbf{Edge}} = 0$.** The model parameters are $\theta_1 = 0.125\pi$, $\theta_2 = 0.25\pi$, $\theta_3 = 0.5\pi$, and $\theta_4 = 0.25\pi$, resulting in $\sum c_i = 0$. **(a)** Experimentally measured band diagram of the lattice. **(b)** Numerically simulated band diagram. **(c)** Dispersion spectra derived from the eigenvalues of the Floquet operator $U_{F,N}$.

## DISCRETE-STEP FLOQUET OPERATORS AND EIGENVECTORS IN RECIPROCAL SPACE

Since the four-step model exhibits double periodicity – spatial (every two sites $n$) and temporal (every four-time steps $m$)–, we can apply the following Floquet-Bloch ansatz to Eq. S8:

$$\begin{pmatrix} \alpha(n,m) \\ \beta(n,m) \end{pmatrix} = \begin{pmatrix} \tilde{\alpha}(k,\varphi) \\ \tilde{\beta}(k,\varphi) \end{pmatrix} e^{i\frac{Em}{4}} e^{i\frac{kn}{2}} \tag{S29}$$

we can rewrite Equation S8 as,

$$e^{iE} \begin{pmatrix} \tilde{\alpha}(k,\varphi) \\ \tilde{\beta}(k,\varphi) \end{pmatrix} = \tilde{U}_F \begin{pmatrix} \tilde{\alpha}(k,\varphi) \\ \tilde{\beta}(k,\varphi) \end{pmatrix} \tag{S30}$$

where $\tilde{U}_F$ is four-step Floquet operator in reciprocal space and Eq. S30 represents eigenvalue equation for our system.

$$\tilde{U}_F(k,\varphi) = \begin{pmatrix} \tilde{u}_1 & \tilde{u}_2 \\ \tilde{u}_3 & \tilde{u}_4 \end{pmatrix} \tag{S31}$$

where,

$$\begin{aligned}
\tilde{u}_1 &= T_1T_2T_3T_4e^{-2ik} - R_2R_4T_1T_3 - R_1R_3T_2T_4 + R_1R_2R_3R_4e^{-2i\varphi} - R_1R_4T_2T_3e^{ik-i\varphi} - R_2R_3T_1T_4e^{-ik+i\varphi} \\
&\quad - R_1R_2T_3T_4e^{-ik-i\varphi} - R_3R_4T_1T_2e^{-ik-i\varphi} \\
\tilde{u}_2 &= R_3T_1T_2T_4i - R_1R_2R_4T_3i + R_1T_2T_3T_4ie^{-2ik} - R_2R_3R_4T_1ie^{-2i\varphi} - R_1R_2R_3T_4ie^{-ik}e^{i\varphi} - R_1R_3R_4T_2ie^{-ik}e^{-i\varphi} \\
&\quad + R_4T_1T_2T_3ie^{ik}e^{-i\varphi} + R_2T_1T_3T_4ie^{-ik}e^{-i\varphi} \\
\tilde{u}_3 &= R_3T_1T_2T_4i - R_1R_2R_4T_3i + R_1T_2T_3T_4ie^{2ik} - R_2R_3R_4T_1ie^{2i\varphi} - R_1R_3R_4T_2ie^{ik}e^{i\varphi} - R_1R_2R_3T_4ie^{ik}e^{-i\varphi} \\
&\quad + R_2T_1T_3T_4ie^{ik}e^{i\varphi} + R_4T_1T_2T_3ie^{-ik}e^{i\varphi} \\
\tilde{u}_4 &= T_1T_2T_3T_4e^{2ik} - R_2R_4T_1T_3 - R_1R_3T_2T_4 + R_1R_2R_3R_4e^{2i\varphi} - R_1R_2T_3T_4e^{ik}e^{i\varphi} - R_3R_4T_1T_2e^{ik}e^{i\varphi} - R_1R_4T_2T_3e^{-ik}e^{i\varphi} \\
&\quad - R_2R_3T_1T_4e^{ik}e^{-i\varphi}
\end{aligned} \tag{S32}$$

The Floquet operator $\tilde{U}_F$ in Equation S31 can also be written in the following compact form:

$$\tilde{U}_F(k,\varphi) = U_0 + U_+e^{ik} + U_{++}e^{2ik} + U_-e^{-ik} + U_{--}e^{-2ik} \tag{S33}$$

To find the corresponding bulk topological invariant, we first check that $\tilde{U}_F(k,\varphi)$ is in the D symmetry class with particle-hole symmetry

$$\mathcal{P}\tilde{U}_F(k,\varphi)\mathcal{P}^{-1} = \tilde{U}_F(-k,-\varphi), \tag{S34}$$

implemented by the anti-unitary operator $\mathcal{P} = \sigma_z K$, being $K$ the complex conjugation operation. This implies that the bulk topological invariant corresponds to the Chern number [2].

### Eigenvalues and eigenvectors

Solving Equation S30 for the eigenvalues of $\tilde{U}_F$ we obtain the solutions of energies of the bands $E_\pm$:

$$E_\pm(k,\varphi) = \pm\cos^{-1}[T_1T_2T_3T_4\cos(2k) - R_2R_4T_1T_3 - R_1R_2T_3T_4\cos(k+\varphi) - R_3R_4T_1T_2\cos(k+\varphi) - R_1R_4T_2T_3\cos(k-\varphi) - R_2R_3T_1T_4\cos(k-\varphi) - R_1R_3T_2T_4 + R_1R_2R_3R_4\cos(2\varphi)], \tag{S35}$$

and the eigenvectors in reciprocal space are given by

$$|\psi\rangle = \begin{pmatrix}\tilde{\alpha}(k,\varphi)\\ \tilde{\beta}(k,\varphi)\end{pmatrix} = \frac{1}{\sqrt{1+|R^\pm|^2}}\begin{pmatrix}1\\ |R^\pm|e^{i\Phi^\pm_{\alpha\beta}}\end{pmatrix}, \tag{S36}$$

where

$$R^\pm(k,\varphi) = \frac{\tilde{\beta}(k,\varphi)}{\tilde{\alpha}(k,\varphi)} = \frac{e^{iE_\pm} - A}{B} = |R^\pm|e^{i\Phi^\pm_{\alpha\beta}} \tag{S37}$$

with

$$\begin{aligned} A &= T_1T_2T_3T_4e^{-2ik} - R_2R_4T_1T_3 - R_1R_2T_3T_4e^{-i(k+\varphi)} - R_3R_4T_1T_2e^{-i(k+\varphi)} - R_1R_3T_2T_4 + R_1R_2R_3R_4e^{-2i\varphi} \\ &\quad - R_1R_4T_2T_3e^{i(k-\varphi)} - R_2R_3T_1T_4e^{-i(k-\varphi)} \\ B &= -R_1R_2R_4T_3i + R_3T_1T_2T_4i - R_1R_3R_4T_2ie^{-i(k+\varphi)} + R_2T_1T_3T_4ie^{-i(k+\varphi)} + R_1T_2T_3T_4ie^{-2ik} - R_2R_3R_4T_1ie^{-2i\varphi} \\ &\quad - R_1R_2R_3T_4ie^{-i(k-\varphi)} + R_4T_1T_2T_3ie^{i(k-\varphi)}. \end{aligned} \tag{S38}$$

## COMPUTATION OF THE WINDING OF THE EDGE OPERATORS

Inspired by Ref. [3], we modify the phase modulators acting on the edge sites (see Fig. S5.**b**) to modify the winding at the boundary of the finite lattice. As we will see below, this intuitive approach allows to easily design the winding $\nu_{\text{Edge}}$. The phase modulators of the left boundary are tuned using the parameter $\boldsymbol{c} \in \mathbb{Z}$ such that $\varphi_{1,0} = \phi_1 = \boldsymbol{c_1}\varphi$, $\varphi_{2,-1} = \phi_2 = \boldsymbol{c_2}\varphi$, $\varphi_{3,0} = \phi_3 = \boldsymbol{c_3}\varphi$ and $\varphi_{4,-1} = \phi_4 = \boldsymbol{c_4}\varphi$. This modifies the initial Floquet operator $U_{F,N}$ to $X_{F,N}$ for the lattice in Fig. S5.**b**. When $\boldsymbol{c_1} = \boldsymbol{c_3} = 1$ and $\boldsymbol{c_2} = \boldsymbol{c_4} = -1$ we get $X_{F,N} = U_{F,N}$, that is, the original finite lattice without any modification Fig. S5.**a**.

To calculate the winding number $\nu_{\text{Edge}}$ associated to the edge of the full Floquet operator $X_{F,N}$, we now need to compute $U_{edge}$. We follow the procedure introduced by Bessho and coworkers in Ref. [3] and express the full Floquet unitary operator $X_{F,N}$ as a product of two unitary operators:

$$X_{F,N} = U_{Edge}U_{F,N} \tag{S39}$$

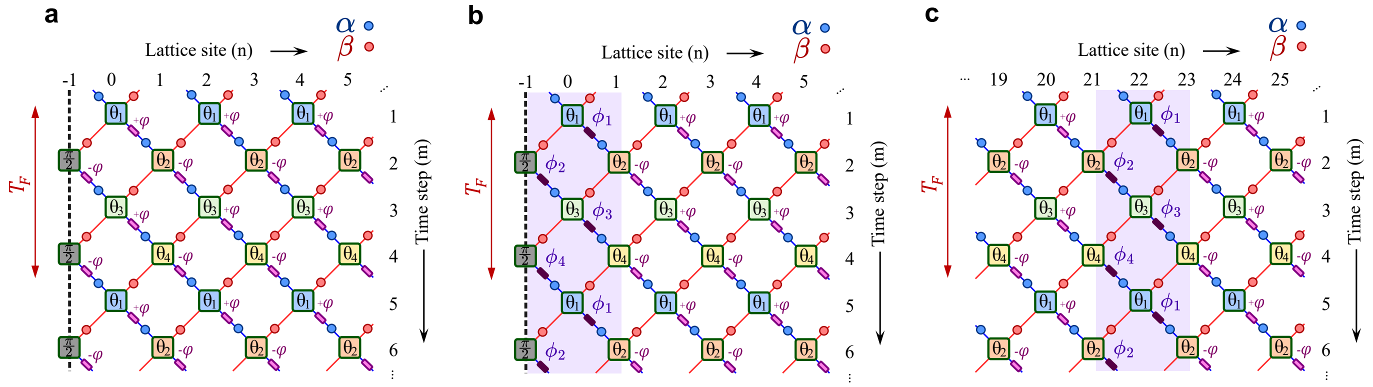


FIG. S5. **a** Discrete-step finite lattice after time demultiplexing of the pulses in the double ring set-up. **b** Discrete-step finite lattice with modified edge operators in the left boundary of the lattice. **c** Discrete-step finite lattice with modified edge operators in the bulk of the lattice.

We remind here that $U_{F,N}$ is the bulk Floquet operator with no modification of the phase modulation at the edges. It is now straightforward to compute $U_{Edge}$:

$$U_{Edge} = X_{F,N}(U_{F,N})^{-1} = \begin{pmatrix} U_1 & U_2 & U_3 & 0 & 0 & 0 & 0 & \\ U_4 & U_5 & U_6 & 0 & 0 & 0 & \iddots & 0 \\ U_7 & U_8 & U_9 & 0 & 0 & \iddots & 0 & 0 \\ 0 & 0 & 0 & I & \iddots & 0 & 0 & 0 \\ 0 & 0 & 0 & \iddots & I & 0 & 0 & 0 \\ 0 & 0 & \iddots & 0 & 0 & I & 0 & 0 \\ 0 & \iddots & 0 & 0 & 0 & 0 & I & 0 \\ & 0 & 0 & 0 & 0 & 0 & 0 & I \end{pmatrix} \tag{S40}$$

where $I$ is the identity matrix and the different blocks are given by:

$$U_1 = \begin{pmatrix} u_{11} & u_{12} \\ u_{13} & u_{14} \end{pmatrix} \tag{S41}$$

$$\begin{aligned}
u_{11} &= e^{i\varphi(c_1+c_4)}R_1^2R_2^2T_3^2 + e^{i\varphi(c_2+c_4+2)}R_1^2R_3^2 + e^{i\varphi(c_1+c_4)}R_2^2T_1^2T_3^2 + e^{i\varphi(c_2+c_4+2)}R_3^2T_1^2 + e^{i\varphi(c_4+1)}T_2^2T_3^2 \\
u_{12} &= -R_3T_3ie^{-2i\varphi}(R_1^2+T_1^2)(R_2^2R_4e^{i\varphi(c_1+c_4)} - R_4e^{i\varphi(c_2+c_4+2)} + R_4T_2^2e^{i\varphi(c_4+1)} - R_2T_2T_4e^{i\varphi(c_1+c_4+2)} + R_2T_2T_4e^{i\varphi(c_4+3)}) \\
u_{13} &= R_3T_3i(R_4e^{i\varphi(c_1+c_3)} - R_4e^{i\varphi(c_2+c_3+2)} - R_4T_2^2e^{i\varphi(c_1+c_3)} + R_2T_2T_4 + R_4T_2^2e^{i\varphi(c_3+1)} - R_2T_2T_4e^{i\varphi(c_1-1)}) \\
u_{14} &= e^{i\varphi(c_1-3)}(R_4^2T_3^2e^{i\varphi(c_2-c_1+c_3+3)} + R_3^2T_2^2T_4^2e^{2i\varphi} + R_3^2R_4^2T_2^2e^{i\varphi(c_3-c_1+2)} + R_2^2R_3^2R_4^2e^{i\varphi(c_3+1)} + R_2^2R_3^2T_4^2e^{-i\varphi(c_1-3)} \\
&\quad + R_2^2T_3^2T_4^2e^{-i\varphi(c_1-3)} + T_2^2T_3^2T_4^2e^{-i\varphi(c_1-3)} - R_2R_3^2R_4T_2T_4 + R_2R_3^2R_4T_2T_4e^{i\varphi(c_3-c_1+4)} + R_2R_3^2R_4T_2T_4e^{-i\varphi(c_1-1)} \\
&\quad - R_2R_3^2R_4T_2T_4e^{i\varphi(c_3+3)}),
\end{aligned} \tag{S42}$$

$$U_2 = \begin{pmatrix} u_{21} & u_{22} \\ u_{23} & u_{24} \end{pmatrix} \tag{S43}$$

$$\begin{aligned}
u_{21} &= R_3T_3e^{-i\varphi}(R_1^2+T_1^2)(R_2^2T_4e^{i\varphi(c_1+c_4)} - T_4e^{i\varphi(c_2+c_4+2)} + T_2^2T_4e^{i\varphi(c_4+1)} + R_2R_4T_2e^{i\varphi(c_1+c_4+2)} - R_2R_4T_2e^{i\varphi(c_4+3)}) \\
u_{22} &= -R_2R_4T_2T_3^2i(e^{c_4i\varphi} - e^{i\varphi(c_1+c_4-1)}) \\
u_{23} &= -ie^{i\varphi(c_1-2)}(R_2R_3^2T_2T_4^2 - R_4T_3^2T_4e^{i\varphi(c_2-c_1+c_3+3)} + R_3^2R_4T_2^2T_4e^{2i\varphi} + R_2R_3^2R_4^2T_2e^{i\varphi(c_3-c_1+4)} - R_3^2R_4T_2^2T_4e^{i\varphi(c_3-c_1+2)} \\
&\quad - R_2R_3^2R_4^2T_2e^{i\varphi(c_3+3)} - R_2^2R_3^2R_4T_4e^{i\varphi(c_3+1)} + R_2^2R_3^2R_4T_4e^{-i\varphi(c_1-3)} - R_2R_3^2T_2T_4^2e^{-i\varphi(c_1-1)} + R_2^2R_4T_3^2T_4e^{-i\varphi(c_1-3)} \\
&\quad + R_4T_2^2T_3^2T_4e^{-i\varphi(c_1-3)}) \\
u_{24} &= R_3T_2T_3e^{-i\varphi}(R_2e^{i\varphi(c_3+1)} - R_2e^{i\varphi(c_1+c_3)} + R_2T_4^2e^{i\varphi(c_1+c_3)} - R_4T_2T_4 - R_2T_4^2e^{i\varphi(c_3+1)} + R_4T_2T_4e^{i\varphi(c_1-1)}),
\end{aligned} \tag{S44}$$

$$U_3 = \begin{pmatrix} R_2T_2T_3^2T_4(e^{i\varphi(c_4+1)} - e^{i\varphi(c_1+c_4)}) & 0 \\ -R_3T_2T_3T_4i(T_2T_4 - R_2R_4e^{i\varphi(c_3+1)} - T_2T_4e^{i\varphi(c_1-1)} + R_2R_4e^{i\varphi(c_1+c_3)}) & 0 \end{pmatrix}, \tag{S45}$$

$$U_4 = \begin{pmatrix} u_{41} & u_{42} \\ u_{43} & u_{44} \end{pmatrix} \tag{S46}$$

$$\begin{aligned}
u_{41} &= R_3T_3T_4e^{i\varphi(c_1+c_3-1)} - R_3T_3T_4e^{i\varphi(c_2+c_3+1)} + R_3T_2^2T_3T_4e^{c_3i\varphi} - R_3T_2^2T_3T_4e^{i\varphi(c_1+c_3-1)} + R_2R_3R_4T_2T_3e^{i\varphi(c_1-2)} \\
&\quad - R_2R_3R_4T_2T_3e^{-i\varphi} \\
u_{42} &= ie^{-3i\varphi}(R_2R_3^2R_4^2T_2 - R_4T_3^2T_4e^{i\varphi(c_2+c_3+2)} + R_2^2R_3^2R_4T_4e^{2i\varphi} + R_2^2R_4T_3^2T_4e^{2i\varphi} + R_4T_2^2T_3^2T_4e^{2i\varphi} - R_2^2R_3^2R_4T_4e^{i\varphi(c_1+c_3)} \\
&\quad + R_2R_3^2T_2T_4^2e^{i\varphi(c_1+c_3+2)} - R_2R_3^2R_4^2T_2e^{i\varphi(c_1-1)} + R_3^2R_4T_2^2T_4e^{i\varphi(c_1+1)} - R_2R_3^2T_2T_4^2e^{i\varphi(c_3+3)} - R_3^2R_4T_2^2T_4e^{i\varphi(c_3+1)}) \\
u_{43} &= -R_2R_4T_2T_3^2i(e^{c_1i\varphi} - e^{i\varphi}) \\
u_{44} &= R_3T_2T_3e^{-i\varphi}(R_2 - R_2e^{i\varphi(c_1-1)} - R_2T_4^2 + R_2T_4^2e^{i\varphi(c_1-1)} + R_4T_2T_4e^{i\varphi(c_1+1)} - R_4T_2T_4e^{2i\varphi}),
\end{aligned} \tag{S47}$$

$$U_5 = \begin{pmatrix} u_{51} & u_{52} \\ u_{53} & u_{55} \end{pmatrix} \tag{S48}$$

$$\begin{aligned}
u_{51} &= e^{-2i\varphi}(T_3^2T_4^2e^{i\varphi(c_2+c_3+2)} + R_2^2R_3^2R_4^2e^{2i\varphi} + R_2^2R_4^2T_3^2e^{2i\varphi} + R_4^2T_2^2T_3^2e^{2i\varphi} + R_2^2R_3^2T_4^2e^{i\varphi(c_1+c_3)} + R_3^2R_4^2T_2^2e^{i\varphi(c_1+1)} \\
&\quad + R_3^2T_2^2T_4^2e^{i\varphi(c_3+1)} - R_2R_3^2R_4T_2T_4 + R_2R_3^2R_4T_2T_4e^{i\varphi(c_1+c_3+2)} + R_2R_3^2R_4T_2T_4e^{i\varphi(c_1-1)} - R_2R_3^2R_4T_2T_4e^{i\varphi(c_3+3)}) \\
u_{52} &= -R_3T_2T_3e^{-2i\varphi}(T_2i + T_2\sin(\varphi(c_1-1)) - T_2i\cos(\varphi(c_1-1)) - T_2T_4^2i + T_2T_4^2ie^{i\varphi(c_1-1)} + R_2R_4T_4ie^{i\varphi(c_3+1)} \\
&\quad - R_2R_4T_4ie^{i\varphi(c_1+c_3)}) \\
u_{53} &= -R_3T_2T_3i(T_2e^{i\varphi(c_1+1)} - T_2e^{2i\varphi} + T_2T_4^2e^{2i\varphi} - R_2R_4T_4 - T_2T_4^2e^{i\varphi(c_1+1)} + R_2R_4T_4e^{i\varphi(c_1-1)}) \\
u_{54} &= R_4^2e^{i\varphi(c_1-1)} - R_4^2 + R_2^2R_4^2 + R_3^2R_4^2 - R_2^2R_4^2e^{i\varphi(c_1-1)} - R_3^2R_4^2e^{i\varphi(c_1-1)} - R_2^2R_3^2R_4^2 + R_2^2R_3^2R_4^2e^{i\varphi(c_1-1)} + 1,
\end{aligned} \tag{S49}$$

$$U_6 = \begin{pmatrix} R_3T_2T_3T_4e^{-i\varphi}(R_4T_2 - R_4T_2e^{i\varphi(c_1-1)} + R_2T_4e^{i\varphi(c_3+1)} - R_2T_4e^{i\varphi(c_1+c_3)}) & 0 \\ R_4T_2^2T_3^2T_4i(e^{c_1i\varphi} - e^{i\varphi}) & 0 \end{pmatrix}, \tag{S50}$$

$$U_7 = \begin{pmatrix} R_2T_2T_3^2T_4(1-e^{c_1i\varphi-i\varphi}) & -R_3T_2T_3T_4ie^{i\varphi(c_1-3)}(R_2R_4 - T_2T_4e^{2i\varphi})(e^{-i\varphi(c_1-1)}-1) \\ 0 & 0 \end{pmatrix}, \tag{S51}$$

$$U_8 = \begin{pmatrix} u_{81} & u_{82} \\ 0 & 0 \end{pmatrix} \tag{S52}$$

$$u_{81} = R_3T_2T_3T_4e^{-i\varphi}(R_2T_4 - R_2T_4e^{i\varphi(c_1-1)} - R_4T_2e^{i\varphi(c_1+1)} + R_4T_2e^{2i\varphi}) \tag{S53}$$

$$u_{82} = -R_4T_2^2T_3^2T_4ie^{-2i\varphi}(e^{c_1i\varphi} - e^{i\varphi}) \quad , \tag{S54}$$

$$U_9 = \begin{pmatrix} u_{91} & 0 \\ 0 & 1 \end{pmatrix} \tag{S55}$$

$$\begin{aligned}
u_{91} &= T_2^2T_3^2 - T_2^2T_3^2T_4^2 + R_1^2R_2^2R_3^2R_4^2 + R_1^2R_2^2R_3^2T_4^2 + R_1^2R_2^2R_4^2T_3^2 + R_1^2R_3^2R_4^2T_2^2 + R_2^2R_3^2R_4^2T_1^2 + R_1^2R_2^2T_3^2T_4^2 \\
&\quad + R_1^2R_3^2T_2^2T_4^2 + R_2^2R_3^2T_1^2T_4^2 + R_2^2R_4^2T_1^2T_3^2 + R_3^2R_4^2T_1^2T_2^2 + R_2^2T_1^2T_3^2T_4^2 + R_3^2T_1^2T_2^2T_4^2 + T_2^2T_3^2T_4^2e^{i\varphi(c_1-1)},
\end{aligned} \tag{S56}$$

***

To compute the invariant associated to the winding of $U_{Edge}$, we use Eq. 2 in the main text:

$$\nu_{\text{Edge}} = \nu[U_{Edge}] = \frac{1}{2\pi}\int_0^{2\pi} d\varphi \ \text{Tr}[U_{\text{Edge}}(\varphi)^{-1}i\partial_\varphi U_{\text{Edge}}(\varphi)]. \tag{S57}$$

To make this computation we note that $U_{Edge}$ is block diagonal with the first block of nine matrices being the only one containing meaningful information. The other blocks are identity matrices in the main diagonal. To compute $\nu_{\text{Edge}}$ we just need to apply Eq. S57 to the first block:

$$U_L \equiv \begin{pmatrix} U_1 & U_2 & U_3 \\ U_4 & U_5 & U_6 \\ U_7 & U_8 & U_9 \end{pmatrix}. \tag{S58}$$

It is straightforward to show that

$$\nu_{\text{Edge}} = \nu[U_{Edge}] = \nu[U_L] = -(\boldsymbol{c_1} + \boldsymbol{c_2} + \boldsymbol{c_3} + \boldsymbol{c_4}) = -\sum_{i=0}^{4} \boldsymbol{c_i}. \tag{S59}$$

This expression shows that the winding of the edge unitary operator can be arbitrarily modified through the design of $\boldsymbol{c_1}$, $\boldsymbol{c_2}$, $\boldsymbol{c_3}$ and $\boldsymbol{c_4}$. A similar description can easily be provided for the right boundary if it is also modified. Unlike

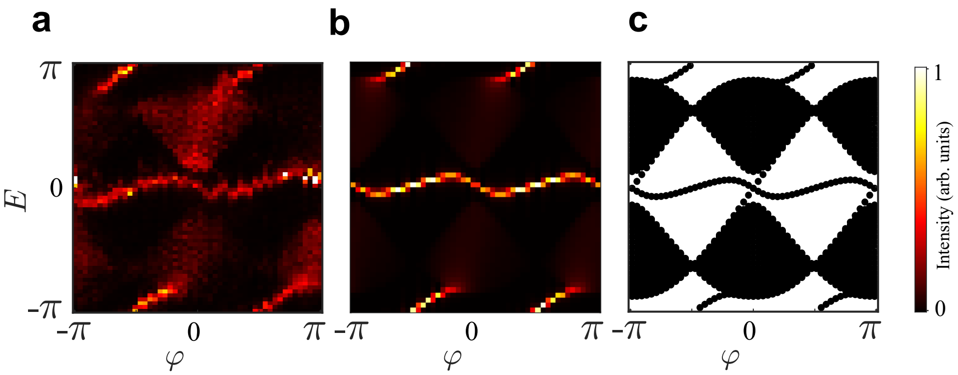


FIG. S6. **Band diagram for a lattice model with Chern number $\mathcal{C}^+$ = -2 and edge winding number $\nu_{\text{Edge}}$ = -2.** The model parameters are $\theta_1 = 0.125\pi$, $\theta_2 = 0.25\pi$, $\theta_3 = 0.5\pi$, and $\theta_4 = 0.25\pi$, resulting in $\sum c_i = 2$. **(a)** Experimentally measured band diagram of the lattice. **(b)** Numerically simulated band diagram. **(c)** Dispersion spectra derived from the eigenvalues of the Floquet operator $X_{F,N}$.

a conventional 2D system we can modify the winding of left boundary without affecting the right boundary since the parametric dimension $\varphi$ in our lattice model has periodic boundary condition.

Let us simplify even further the above general expressions. For a very simple case where we modify only $\boldsymbol{c_4}$ and $\boldsymbol{c_1 = 1,\ c_2 = -1,\ c_3 = 1}$ are unmodified as in original finite lattice, $U_{Edge}$ reduces to,

$$U_{Edge} = \begin{pmatrix} U_1 & 0 & 0 & 0 & 0 & 0 & 0 & \\ 0 & I & 0 & 0 & 0 & 0 & \ddots & 0 \\ 0 & 0 & I & 0 & 0 & \ddots & 0 & 0 \\ 0 & 0 & 0 & I & \ddots & 0 & 0 & 0 \\ 0 & 0 & 0 & \ddots & I & 0 & 0 & 0 \\ 0 & 0 & \ddots & 0 & 0 & I & 0 & 0 \\ 0 & \ddots & 0 & 0 & 0 & 0 & I & 0 \\ & 0 & 0 & 0 & 0 & 0 & 0 & I \end{pmatrix} \tag{S60}$$

where

$$U_1 = \begin{pmatrix} e^{i\varphi(c_4+1)} & 0 \\ 0 & 1 \end{pmatrix} = U_L \tag{S61}$$

The winding number of the edge unitary can be calculated as $\nu_{\text{Edge}} = \nu[U_{Edge}] = \nu[U_L] = -(\boldsymbol{c_4} + 1)$.

The eigenvalues of $X_{F,N}$ for a finite size lattice with Chern number -2 in the lower band and edge winding of -2 at the left boundary are shown in Fig. S6.**c**. In the $E = 0$ gap we observe the cancellation of the left chiral edges, while the right chiral edges associated to the Chern bulk topology are still present at the right edge. The edge mode band traversing the $E = \pi$ gap arises fully from the winding of $U_{Edge}$ The corresponding experimental results are shown in Fig. S6.**a**.

## COMPUTATION OF THE WINDING OF THE STRIPE OPERATORS IN THE BULK

For a special case of inducing chiral localised modes within the bulk of the lattice we select a cell far from the edges ($n_b = 22$) and implement locally the Floquet sequence of phases such that $\varphi_{1,n_b} = \phi_1 = \phi_1^{n_b} = \boldsymbol{c_1}\varphi,\ \varphi_{2,n_b-1} = \phi_2 = \phi_2^{n_b} = \boldsymbol{c_2}\varphi,\ \varphi_{3,n_b} = \phi_3 = \phi_3^{n_b} = \boldsymbol{c_3}\varphi$ and $\varphi_{4,n_b-1} = \phi_4 = \phi_4^{n_b} = \boldsymbol{c_4}\varphi$ similar to the previous case. This modifies the initial Floquet operator $U_{F,N}$ to $X^b_{F,N}$ of the lattice in Fig. S5.**c** and the corresponding stripe operator to $U_{n_b}$ such that,

$$U_{n_b} = X^b_{F,N}(U_{F,N})^{-1} = \begin{pmatrix} I & 0 & 0 & 0 & 0 & 0 & 0 & 0 & 0 & 0 \\ 0 & \ddots & 0 & 0 & 0 & 0 & 0 & 0 & 0 & 0 \\ 0 & 0 & I & 0 & 0 & 0 & 0 & 0 & 0 & 0 \\ 0 & 0 & 0 & U_1 & U_2 & U_3 & U_4 & 0 & 0 & 0 \\ 0 & 0 & 0 & U_5 & U_6 & U_7 & U_8 & 0 & 0 & 0 \\ 0 & 0 & 0 & U_9 & U_{10} & U_{11} & U_{12} & 0 & 0 & 0 \\ 0 & 0 & 0 & U_{13} & U_{14} & U_{15} & U_{16} & 0 & 0 & 0 \\ 0 & 0 & 0 & 0 & 0 & 0 & 0 & I & 0 & 0 \\ 0 & 0 & 0 & 0 & 0 & 0 & 0 & 0 & \ddots & 0 \\ 0 & 0 & 0 & 0 & 0 & 0 & 0 & 0 & 0 & I \end{pmatrix} \tag{S62}$$

where $I$ is the identity matrix and the different blocks are given by:

$$U_1 = \begin{pmatrix} 1 & 0 \\ 0 & T_4^2(e^{i\varphi(1+c_2)} - 1) + T_3^2T_4^2(T_2^2 - e^{i\varphi(1+c_2)} + e^{i\varphi(c_1-1)} - T_2^2e^{i\varphi(c_1-1)}) + 1 \end{pmatrix} \tag{S63}$$

$$U_2 = \begin{pmatrix} 0 & 0 \\ u_{21} & u_{22} \end{pmatrix} \tag{S64}$$

$$\begin{aligned} u_{21} = &-\frac{\sin(2\theta_4)}{8}[2ie^{i\varphi(c_2+2)} - 3ie^{i\varphi} + ie^{c_1 i\varphi} - ie^{c_1 i\varphi}\cos(2\theta_2) + ie^{c_1 i\varphi}\cos(2\theta_3) + ie^{i\varphi}\cos(2\theta_2) + ie^{i\varphi}\cos(2\theta_3) \\ &- 2ie^{i\varphi(c_2+2)}\cos(2\theta_3) - ie^{c_1 i\varphi}\cos(2\theta_2)\cos(2\theta_3) + ie^{i\varphi}\cos(2\theta_2)\cos(2\theta_3)] \\ u_{22} = &-R_3T_3T_4e^{-i\varphi}(R_4T_2^2 - R_4e^{i\varphi(1+c_2)} + R_4(\cos(\varphi(c_1-1)) + i\sin(\varphi(c_1-1))) - R_4T_2^2e^{i\varphi(c_1-1)} - R_2T_2T_4e^{i\varphi(1+c_1)} \\ &+ R_2T_2T_4e^{2i\varphi}) \end{aligned} \tag{S65}$$

$$U_3 = \begin{pmatrix} 0 & 0 \\ u_{31} & u_{32} \end{pmatrix} \tag{S66}$$

$$\begin{aligned} u_{31} &= R_3T_3T_4(T_4ie^{i\varphi(1+c_2)} - T_4ie^{i\varphi(c_1-1)} - T_2^2T_4i + T_2^2T_4ie^{i\varphi(c_1-1)} + R_2R_4T_2ie^{2i\varphi} - R_2R_4T_2ie^{i\varphi(1+c_1)}) \\ u_{32} &= R_2R_4T_2T_3^2T_4(e^{i\varphi(c_1-1)} - 1) \end{aligned} \tag{S67}$$

$$U_4 = \begin{pmatrix} 0 & 0 \\ -R_2T_2T_3^2T_4^2(ie^{i\varphi} - ie^{c_1 i\varphi}) & 0 \end{pmatrix} \tag{S68}$$

$$U_5 = \begin{pmatrix} 0 & R_4T_4ie^{c_4 i\varphi}(e^{i\varphi(c_2+1)} - 1 + T_2^2T_3^2 + T_3^2e^{i\varphi(c_1-1)} - T_3^2e^{i\varphi(c_2+1)} - T_2^2T_3^2e^{i\varphi(c_1-1)}) \\ 0 & R_3T_3T_4e^{-i\varphi}(R_4e^{(2+c_2+c_3)i\varphi} - R_4e^{(c_1+c_3)i\varphi} + R_4T_2^2e^{(c_1+c_3)i\varphi} - R_2T_2T_4 - R_4T_2^2e^{(1+c_3)i\varphi} + R_2T_2T_4e^{(c_1-1)i\varphi}) \end{pmatrix} \tag{S69}$$

$$U_6 = \begin{pmatrix} u_{61} & u_{62} \\ u_{63} & u_{64} \end{pmatrix} \tag{S70}$$

$$\begin{aligned} u_{61} = &\, e^{(c_4+1)i\varphi} - R_2^2R_4^2e^{(c_4+1)i\varphi} - R_3^2R_4^2e^{(c_4+1)i\varphi} + R_2^2R_4^2e^{(c_1+c_4)i\varphi} + R_2^2R_3^2R_4^2e^{(c_4+1)i\varphi} + R_3^2R_4^2e^{(c_2+c_4+2)i\varphi} \\ &- R_2^2R_3^2R_4^2e^{(c_1+c_4)i\varphi} \\ u_{62} = &\, iR_3T_3(e^{(c_2+c_4)i\varphi} - e^{(c_1+c_4-2)i\varphi} - T_4^2e^{(c_2+c_4)i\varphi} - T_2^2e^{(c_4-1)i\varphi} + T_2^2T_4^2e^{(c_4-1)i\varphi} + T_2^2e^{(c_1+c_4-2)i\varphi} + T_4^2e^{(c_1+c_4-2)i\varphi} \\ &- T_2^2T_4^2e^{(c_1+c_4-2)i\varphi}) - iR_2R_3R_4T_2T_3T_4(e^{(c_4+1)i\varphi} - e^{c_1+c_4)i\varphi}) \\ u_{63} = &\, \frac{i}{2}\sin(2\theta_3)(e^{(c_1+c_3)i\varphi} - e^{(c_2+c_3+2)i\varphi}) - iR_3T_3(T_2^2 + T_4^2)e^{(c_1+c_3)i\varphi} + iR_3T_3(T_2^2e^{(c_3+1)i\varphi} + T_4^2e^{(c_2+c_3+2)i\varphi} \\ &- T_2^2T_4^2e^{(c_3+1)i\varphi} + T_2^2T_4^2e^{(c_1+c_3)i\varphi}) + iR_2R_3R_4T_2T_3T_4(1 - e^{(c_1-1)i\varphi}) \\ u_{64} = &\, e^{(c_1-3)i\varphi}(R_2^2R_3^2T_4^2e^{(3-c_1)i\varphi} + R_2^2T_3^2T_4^2e^{(3-c_1)i\varphi} + T_2^2T_3^2T_4^2e^{(3-c_1)i\varphi} + R_3^2T_2^2T_4^2e^{2i\varphi} + R_3^2R_4^2T_2^2e^{(c_3-c_1+2)i\varphi} \\ &+ R_2^2R_4^2T_3^2e^{(c_2+c_3-c_1+3)i\varphi} + R_4^2T_2^2T_3^2e^{(c_2+c_3-c_1+3)i\varphi} + R_2^2R_3^2R_4^2e^{(c_3+1)i\varphi} \\ &+ R_2R_3^2R_4T_2T_4(-1 + e^{(c_3-c_1+4)i\varphi} + e^{(1-c_1)i\varphi} - e^{(c_3+3)i\varphi})) \end{aligned} \tag{S71}$$

$$U_7 = \begin{pmatrix} u_{71} & u_{72} \\ u_{73} & u_{74} \end{pmatrix} \tag{S72}$$

$$\begin{aligned}
u_{71} = & -R_3T_3(\frac{\sin(2\theta_2)e^{i\varphi(2+c_4)}}{2} - R_2T_2e^{i\varphi(1+c_1+c_4)} + R_4T_4e^{\varphi(i+c_2i+c_4i)} - R_4T_4e^{i\varphi(c_1-1+c_4)} + R_2T_2T_4^2e^{i\varphi(1+c_1+c_4)} \\
& - R_2T_2T_4^2e^{i\varphi(2+c_4)} + R_4T_2^2T_4e^{i\varphi(c_1-1+c_4)} - R_4T_2^2T_4e^{c_4i\varphi}) \\
u_{72} = & R_2T_2T_3^2ie^{i\varphi(c_1-1+c_4)}(T_4^2-1)(e^{i\varphi(1-c_1)}-1) - ie^{-i\varphi(2-c_1)}(R_2R_3^2T_2T_4^2 + R_3^2R_4T_2^2T_4e^{2i\varphi} + R_2R_3^2R_4^2T_2e^{i\varphi(4-c_1+c_3)} \\
& - R_3^2R_4T_2^2T_4e^{i\varphi(2-c_1+c_3)} \\
u_{73} = & \quad -R_2^2R_4T_3^2T_4e^{i\varphi(3-c_1+c_2+c_3)} - R_4T_2^2T_3^2T_4e^{i\varphi(3-c_1+c_2+c_3)} - R_2^2R_3^2R_4T_4e^{i\varphi(1+c_3)} - R_2R_3^2T_2T_4^2e^{i\varphi(1-c_1)} \\
& - R_2R_3^2R_4^2T_2e^{i\varphi(3+c_3)} + R_2^2R_3^2R_4T_4e^{i\varphi(3-c_1)} + R_2^2R_4T_3^2T_4e^{i\varphi(3-c_1)} + R_4T_2^2T_3^2T_4e^{i\varphi(3-c_1)}) \\
u_{74} = & -R_3T_2T_3e^{-i\varphi}(R_2e^{i\varphi(c_1+c_3)} - R_2e^{i\varphi(1+c_3)} - R_2T_4^2e^{i\varphi(c_1+c_3)} + R_4T_2T_4 + R_2T_4^2e^{i\varphi(1+c_3)} - R_4T_2T_4e^{i\varphi(c_1-1)})
\end{aligned} \tag{S73}$$

$$U_8 = \begin{pmatrix} R_2R_4T_2T_3^2T_4(e^{i\varphi(1+c_4)} - e^{i\varphi(c_1+c_4)}) & 0 \\ -R_3T_2T_3T_4(T_2T_4i + R_2R_4ie^{i\varphi(c_1+c_3)} - R_2R_4ie^{i\varphi(1+c_3)} - T_2T_4ie^{i\varphi(c_1-1)}) & 0 \end{pmatrix} \tag{S74}$$

$$U_9 = \begin{pmatrix} 0 & u_{91} \\ 0 & u_{92} \end{pmatrix} \tag{S75}$$

$$\begin{aligned}
u_{91} &= R_3T_3T_4^2i(T_2^2e^{i\varphi(c_3-1)} - e^{i\varphi(c_2+c_3)} + e^{i\varphi(c_1+c_3-2)} - T_2^2e^{i\varphi(c_1+c_3-2)}) - R_2R_3R_4T_2T_3T_4i(e^{-2i\varphi} - e^{i\varphi(c_1-3)}) \\
u_{92} &= R_2R_4T_2T_3^2T_4(e^{i\varphi(c_1-1)} - 1)
\end{aligned} \tag{S76}$$

$$U_{10} = \begin{pmatrix} u_{101} & u_{102} \\ u_{103} & u_{104} \end{pmatrix} \tag{S77}$$

$$\begin{aligned}
u_{101} = & R_2R_3T_2T_3(T_4^2-1)e^{-i\varphi} + R_2R_3T_2T_3e^{(c_1-2)i\varphi} + R_3R_4T_2^2T_3T_4(e^{c_3i\varphi} - e^{(c_1+c_3-1)i\varphi}) \\
& + R_3R_4T_3T_4(e^{(c_1+c_3-1)i\varphi} - e^{(c_2+c_3+1)i\varphi}) \\
u_{102} = & ie^{-3i\varphi}(R_2R_3^2R_4^2T_2(1-e^{c_1i\varphi}) + R_2^2R_3^2R_4T_4(e^{2i\varphi} - e^{(c_1+c_3)i\varphi}) + R_2^2R_4T_3^2T_4e^{2i\varphi}(1-e^{(c_2+c_3-2)i\varphi}) \\
& + R_4T_2^2T_3^2T_4e^{2i\varphi}(1-e^{(c_2+c_3-2)i\varphi}) + R_2R_3^2T_2T_4^2(e^{(2+c_1+c_3)i\varphi} - e^{(3+c_3)i\varphi}) + R_3^2R_4T_2^2T_4(e^{(1+c_1)i\varphi} - e^{(1+c_3)i\varphi})) \\
u_{103} = & R_2T_2T_3^2i(T_4^2-1)(e^{c_1i\varphi} - e^{i\varphi}) \\
u_{104} = & R_3T_2T_3e^{-i\varphi}(R_2(1-e^{(c_1-1)i\varphi})(1-T_4^2) - R_4T_2T_4(e^{2i\varphi} - e^{(1+c_1)i\varphi}))
\end{aligned} \tag{S78}$$

$$U_{11} = \begin{pmatrix} u_{111} & u_{112} \\ u_{113} & u_{114} \end{pmatrix} \tag{S79}$$

$$\begin{aligned}
u_{111} = & e^{-2i\varphi}(R_2^2R_3^2R_4^2e^{2i\varphi} + R_2^2R_4^2T_3^2e^{2i\varphi} + R_4^2T_2^2T_3^2e^{2i\varphi} + R_2^2T_3^2T_4^2e^{i\varphi(2+c_2+c_3)} + T_2^2T_3^2T_4^2e^{i\varphi(2+c_2+c_3)} \\
& + R_2^2R_3^2T_4^2e^{i\varphi(c_1+c_3)} + R_3^2R_4^2T_2^2e^{i\varphi(1+c_1)} + R_3^2T_2^2T_4^2e^{i\varphi(1+c_3)} - R_2R_3^2R_4T_2T_4 + R_2R_3^2R_4T_2T_4e^{i\varphi(2+c_1+c_3)} \\
& + R_2R_3^2R_4T_2T_4e^{i\varphi(c_1-1)} - R_2R_3^2R_4T_2T_4e^{i\varphi(3+c_3)}) \\
u_{112} = & -R_3T_2T_3e^{-2i\varphi}(T_2i + T_2(\sin(\varphi(c_1-1)) - i\cos(\varphi(c_1-1))) - T_2T_4^2i + T_2T_4^2ie^{i\varphi(c_1-1)} - R_2R_4T_4ie^{i\varphi(c_1+c_3)} \\
& + R_2R_4T_4ie^{i\varphi(1+c_3)}) \\
u_{113} = & -R_3T_2T_3(T_2ie^{i\varphi(1+c_1)} - T_2ie^{2i\varphi} + T_2T_4^2ie^{2i\varphi} - R_2R_4T_4i - T_2T_4^2ie^{i\varphi(1+c_1)} + R_2R_4T_4ie^{i\varphi(c_1-1)}) \\
u_{114} = & R_4^2e^{i\varphi(c_1-1)} - R_4^2 + R_2^2R_4^2 + R_3^2R_4^2 - R_2^2R_3^2R_4^2 - R_2^2R_4^2e^{i\varphi(c_1-1)} - R_3^2R_4^2e^{i\varphi(c_1-1)} + R_2^2R_3^2R_4^2e^{i\varphi(c_1-1)} + 1
\end{aligned} \tag{S80}$$

$$U_{12} = \begin{pmatrix} R_3T_2T_3T_4e^{-i\varphi}(R_4T_2 + R_2T_4e^{i\varphi(1+c_3)} - R_4T_2e^{i\varphi(c_1-1)} - R_2T_4e^{i\varphi(c_1+c_3)}) & 0 \\ -R_4T_2^2T_3^2T_4i(e^{i\varphi} - e^{c_1 i\varphi}) & 0 \end{pmatrix} \tag{S81}$$

$$U_{13} = \begin{pmatrix} 0 & R_2T_2T_3^2T_4^2i(e^{-i\varphi} - e^{(c_1-2)i\varphi}) \\ 0 & 0 \end{pmatrix} \tag{S82}$$

$$U_{14} = \begin{pmatrix} R_2R_4T_2T_3^2T_4(1 - e^{i\varphi(c_1-1)}) & -iR_3T_2T_3T_4e^{-i\varphi(3-c_1)}(R_2R_4 - T_2T_4e^{2i\varphi})(e^{i\varphi(1-c_1)} - 1) \\ 0 & 0 \end{pmatrix} \tag{S83}$$

$$U_{15} = \begin{pmatrix} R_3T_2T_3T_4e^{-i\varphi}(R_2T_4 - R_4T_2e^{i\varphi(1+c_1)} - R_2T_4e^{i\varphi(c_1-1)} + R_4T_2e^{2i\varphi}) & R_4T_2^2T_3^2T_4i(e^{-i\varphi} - e^{i\varphi(c_1-2)}) \\ 0 & 0 \end{pmatrix} \tag{S84}$$

$$U_{16} = \begin{pmatrix} u_{161} & 0 \\ 0 & 1 \end{pmatrix} \tag{S85}$$

$$\begin{aligned} u_{161} = {} & T_2^2T_3^2 - T_2^2T_3^2T_4^2 + R_1^2R_2^2R_3^2R_4^2 + R_1^2R_2^2R_3^2T_4^2 + R_1^2R_2^2R_4^2T_3^2 + R_1^2R_3^2R_4^2T_2^2 + R_2^2R_3^2R_4^2T_1^2 + R_1^2R_2^2T_3^2T_4^2 + R_1^2R_3^2T_2^2T_4^2 \\ & + R_2^2R_3^2T_1^2T_4^2 + R_2^2R_4^2T_1^2T_3^2 + R_3^2R_4^2T_1^2T_2^2 + R_2^2T_1^2T_3^2T_4^2 + R_3^2T_1^2T_2^2T_4^2 + T_2^2T_3^2T_4^2e^{-i\varphi(1-c_1)} \end{aligned} \tag{S86}$$

***

The stripe operator $U_{n_b}$ is intrinsically linked to the edge operator $U_{Edge}$. As illustrated in Figure S5, when we apply this particular stripe pattern of phase modulations to the system at an edge, $U_{n_b}$ transforms into $U_{Edge}$. To compute the invariant associated to the winding of $U_{n_b}$ we use the Eq. S57. Since the winding is in the bulk we note that in the block diagonal $U_{n_b}$ the sixteen matrices containing the meaningful information of the winding is inside the $U_{n_b}$ unlike when we had winding in the edge. Since all other blocks are identity matrices in the main diagonal the winding can be calculated using this block of sixteen matrices:

$$U_B \equiv \begin{pmatrix} U_1 & U_2 & U_3 & U_4 \\ U_5 & U_6 & U_7 & U_8 \\ U_9 & U_{10} & U_{11} & U_{12} \\ U_{13} & U_{14} & U_{15} & U_{16} \end{pmatrix}. \tag{S87}$$

It is straightforward to show that the winding number of the stripe unitary inside the bulk is,

$$\nu_{n_b} = \nu[U_{n_b}] = \nu[U_B] = -(\boldsymbol{c_1} + \boldsymbol{c_2} + \boldsymbol{c_3} + \boldsymbol{c_4}) = -\sum_{i=0}^{4} \boldsymbol{c_i}. \tag{S88}$$

This expression shows that the winding of the stripe unitary operator can be arbitrarily modified through the design of $\boldsymbol{c_1}$, $\boldsymbol{c_2}$, $\boldsymbol{c_3}$ and $\boldsymbol{c_4}$ even inside the bulk.

Again when we simplify even further the above general expressions for a very simple case where we modify only $\boldsymbol{c_4}$ and $\boldsymbol{c_1 = 1}$, $\boldsymbol{c_2 = -1}$, $\boldsymbol{c_3 = 1}$ are unmodified as in original finite lattice, $U_{n_b}$ reduces to,

$$U_{n_b} = \begin{pmatrix} I & 0 & 0 & 0 & 0 & 0 & 0 & 0 \\ 0 & \ddots & 0 & 0 & 0 & 0 & 0 & 0 \\ 0 & 0 & I & 0 & 0 & 0 & 0 & 0 \\ 0 & 0 & 0 & U_1 & 0 & 0 & 0 & 0 \\ 0 & 0 & 0 & 0 & I & 0 & 0 & 0 \\ 0 & 0 & 0 & 0 & 0 & I & 0 & 0 \\ 0 & 0 & 0 & 0 & 0 & 0 & \ddots & 0 \\ 0 & 0 & 0 & 0 & 0 & 0 & 0 & I \end{pmatrix} \tag{S89}$$

where

$$U_1 = \begin{pmatrix} e^{i\varphi(c_4+1)} & 0 \\ 0 & 1 \end{pmatrix} \tag{S90}$$

The winding number of the stripe unitary inside the bulk can be calculated as $\nu_{n_b} = \nu[U_{n_b}] = -(\boldsymbol{c_4} + 1)$. The corresponding experimental results of bulk localised modes are shown in Fig.5 of the main text when the pulse injection is at the site $n_b = 22$ in the $\alpha$ ring for lattice in Fig. S5.**c**.

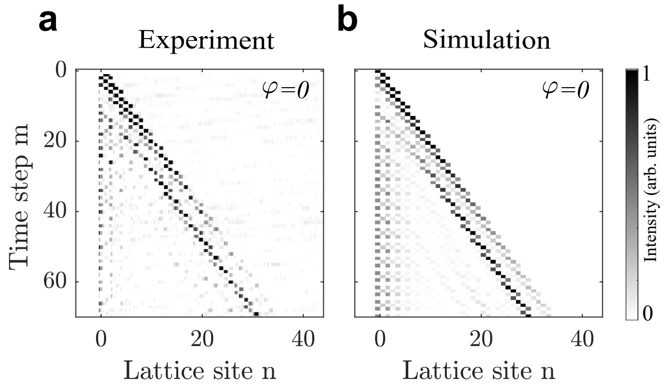


FIG. S7. **Spatio-temporal dynamics in a lattice model with Chern number $\mathcal{C}^+$ = -2 and edge winding number $\nu_{\mathbf{Edge}}$ = 0.** The lattice parameters are $\theta_1 = 0.125\pi$, $\theta_2 = 0.25\pi$, $\theta_3 = 0.5\pi$, and $\theta_4 = 0.25\pi$. **a** Experimentally measured spatio-temporal dynamics of the $\alpha$ ring when a single site at the boundary is excited. **b** Corresponding numerical simulation of the spatio-temporal dynamics.

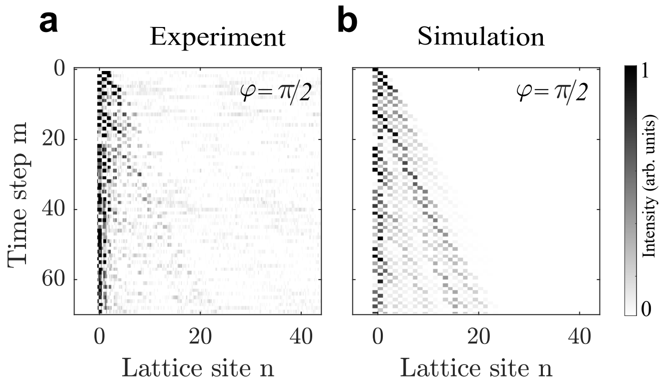


FIG. S8. **Spatio-temporal dynamics in a lattice model with Chern number $\mathcal{C}^+$ = 0 and edge winding number $\nu_{\mathbf{Edge}}$ = -1.** The lattice parameters are $\theta_1 = 0.125\pi$, $\theta_2 = 0.25\pi$, $\theta_3 = 0.438\pi$, and $\theta_4 = 0.438\pi$. **a** Experimentally measured spatio-temporal dynamics of the $\alpha$ ring when a single site at the boundary is excited. **b** Corresponding numerical simulation of the spatio-temporal dynamics.

## EDGE MODES IN REAL SPACE

To generate edge modes in real space precise values for the variable beamsplitter and phase modulator were chosen. The lattice was made with fully reflecting edges ($\theta = \pi/2$) as shown in Fig. S5.**a**.

The presence of edge modes is readily visible in the experiments and simulations via the localisation of light at the edge regions. Two examples are displayed in Figs. S7 and S8. In Fig. S7, we observe edge states in a lattice with Chern number of -2 in the upper band and $\nu_{\text{Edge}} = 0$. In this case the edge states arise solely from the bulk Chern topology. Figure S8 shows the situation of a lattice model with trivial bulk topology and $\nu_{\text{Edge}} = -1$. In this case, the edge states appear solely as a consequence of the nontrivial winding of $U_{Edge}$.

* These authors contributed equally.
† Present address: Quandela, 7 Rue Léonard de Vinci, 91300 Massy, France
‡ a.gomez.leon@csic.es
§ alberto.amo-garcia@univ-lille.fr

[1] M. Blanco de Paz, C. Devescovi, G. Giedke, J. J. Saenz, M. G. Vergniory, B. Bradlyn, D. Bercioux, and A. García-Etxarri, Advanced Quantum Technologies **3**, 1900117 (2020).
[2] S. Ryu, A. P. Schnyder, A. Furusaki, and A. W. W. Ludwig, New Journal of Physics **12**, 065010 (2010).
[3] T. Bessho, K. Mochizuki, H. Obuse, and M. Sato, Phys. Rev. B **105**, 094306 (2022).
